# Supplementary material for: Detectability and global observer design for 2D Navier-Stokes equations with uncertain inputs
Source: arXiv:2110.07738 source file (2023-03-30)
Supplement: Supplementary file 1 [file appendix.tex]

\begin{proof}
Take $\vu=\bigl[
\begin{smallmatrix}u & v
\end{smallmatrix}
\bigr]\in [H_p^2(\Omega)]^2$. By Sobolev embedding theorems (see~\cite[Th.11.3.14]{Hutson1980}) $H^2(\Omega)$ is continuously embedded into the space of continuous functions $C(\Omega)$ hence the vector-function $\vu$ is continuous. Since $\vu$ is also periodic by Weierstrass approximation theorem~\cite[Corollary 3.1.11.]{Grafakos2008} $\vu$ can be represented as a uniform limit of its Fourier series:
\textcolor{blue}{
\begin{equation}
  \label{eq:u-FS}
\lim_{N\to\infty}\sup_{x\in\Omega}\|\vu(\vx)-\sum_{\|\vk\|_{\R^2} \le N}\bigl[
\begin{smallmatrix}
  u_{\vk}&v_{\vk}
\end{smallmatrix}
\bigr] \ee^{2\pi\ii \frac{\vk}{\vL}\cdot \vx}\|_{\R^2}= 0
\end{equation}}
with $u_{\vk}$ and $v_{\vk}$ being complex conjugates of $u_{-\vk}$ and $v_{-\vk}$ (since $\vu$ is real-valued), and
$u_{\vk}=(\ll_1\ll_2)^{-1}\int_\Omega e_1\cdot \vu(\vx)\ee^{-2\pi\ii \frac{\vk}{\vL}\cdot \vx} d\vx$,
and $v_{\vk}$ defined as $u_{\vk}$ but with $e_2$, provided $e_{1,2}$ -- canonical basis of $\R^2$. We have:
\begin{align}
  \|\vu(\vx)\|_{\R^2}&\le \|\vu(\vx)-\sum_{\|\vk\|_{\R^2} \le N}\bigl[
\begin{smallmatrix}
  u_{\vk}&v_{\vk}
\end{smallmatrix}
\bigr] \ee^{2\pi\ii \frac{\vk}{\vL}\cdot \vx}\|_{\R^2}     \label{eq:uxupb}\\
&+\sum_{\|\vk\|_{\R^2}\le N} (|u_{\vk}|_{\C}^2 + |v_{\vk}|_{\C}^2)^{\frac12}
|\ee^{2\pi\ii \frac{\vk}{\vL}\cdot \vx}|_{\C}\\
                   &\le \sum_{\vk\in\Z^2} (|u_{\vk}|_{\C}^2 + |v_{\vk}|_{\C}^2)^{\frac12}\label{eq:ul1}
\end{align}
To get~\eqref{eq:ul1} one sends $N\to\infty$, invokes~\eqref{eq:u-FS} and recalls that $|\ee^{2\pi\ii \frac{\vk}{\vL}\cdot \vx}|_{\C}=1$ and that $\vu\in L^2(\Omega)^2$, as $\vu$ is continuous, hence the series in~\eqref{eq:ul1} is converging.

Let us compute $L^2$-norms of $\vu$, $\nabla\vu=\bigl[
\begin{smallmatrix}
  \nabla u\\\nabla v
\end{smallmatrix}\bigr]
$ and $\Delta\vu = \bigl[
\begin{smallmatrix}
  \Delta u\\\Delta v
\end{smallmatrix}\bigr]$, i.e. $ \|\vu\|^2_{L^2} = \|u\|^2_{L^2}+ \|v\|^2_{L^2}$, $ \|\nabla \vu\|^2_{L^2} = \|\nabla u\|^2_{L^2}+ \|\nabla v\|^2_{L^2}$, $ \|\Delta \vu\|^2_{L^2} = \|\Delta u\|^2_{L^2}+ \|\Delta v\|^2_{L^2}$. To this end we recall Parseval's identity, and classical relations between the smoothness of a function and the decay of its Fourier coefficients (see~\cite[Theorem 3.2.9]{Grafakos2008}), which allow to differentiate Fourier series of a function of $H^2$-class (e.g.~\cite[p.182]{Grafakos2008}) to compute norms of $\nabla\vu$ and $\Delta\vu$:
\begin{align}
    \|\vu\|^2_{L^2}&= \ll_1\ll_2 \sum_{\vk\in\Z^2} (|u_{k_1}|^2_\C +|u_{k_2}|^2_\C), \label{eq:u-l2}
\\
  \|\nabla \vu\|_{L^2}^2 &= 4\pi^2\ll_1\ll_2\sum_{\|\vk\|_{\R^2}\in\Z^2} \|\frac{\vk}{\vL}\|^2_{\R^2}(|u_{\vk}|_{\C}^2 + |v_{\vk}|_{\C}^2),\\
   \|\Delta \vu\|_{L^2}^2 &= 16\pi^4\ll_1\ll_2\sum_{\|\vk\|_{\R^2}\in\Z^2} \|\frac{\vk}{\vL}\|^4_{\R^2}(|u_{\vk}|_{\C}^2 + |v_{\vk}|_{\C}^2). \label{eq:u-Lap}
\end{align}

Now we break the series in~\eqref{eq:ul1} into a finite sum and the remainder:
\begin{align*}
  \|\vu(\vx)\|_{\R^2}&\le \sum_{\|\vk\|_{\R^2}\le \gamma} \frac{\bigl(\ll_1\ll_2 (1+ 4\pi^2 \|\frac{\vk}{\vL}\|^2_{\R^2}) (|u_{\vk}|_{\C}^2 + |v_{\vk}|_{\C}^2)\bigr)^{\frac12}}{(\ll_1\ll_2 + 4\pi^2\ll_1\ll_2 \|\frac{\vk}{\vL}\|^2_{\R^2})^\frac12}\\
   &+\sum_{\|\vk\|_{\R^2}> \gamma}\frac{4\pi^2\sqrt{\ll_1\ll_2}\|\frac{\vk}{\vL}\|^2_{\R^2}}{4\pi^2\sqrt{\ll_1\ll_2}\|\frac{\vk}{\vL}\|^2_{\R^2}} (|u_{\vk}|_{\C}^2 + |v_{\vk}|_{\C}^2)^{\frac12}\\
\end{align*}
and make use of~\eqref{eq:u-l2}-\eqref{eq:u-Lap} to derive~\eqref{eq:AgmoN}:
\begin{align*}
   \|\vu(\vx)\|_{\R^2}&\le \|\vu\|_{H^1}\left(\sum_{\|\vk\|_{\R^2}\le \gamma}(\ll_1\ll_2 + 4\pi^2\ll_1\ll_2 \|\frac{\vk}{\vL}\|^2_{\R^2})^{-1}\right)^{\frac12}\\
   &+\|\Delta\vu\|_{L^2} \left(\sum_{\|\vk\|_{\R^2}> \gamma}(16\pi^4\ll_1\ll_2\|\frac{\vk}{\vL}\|^4_{\R^2})^{-1}\right)^{\frac12}\\
   &\le \|\vu\|_{H^1} \left(\int_{x_1^2+x_2^2\le \gamma} \frac{dx_1dx_2}{\ll_1\ll_2 + 4\pi^2\ll_1\ll_2 \|\frac{\vx}{\vL}\|^2_{\R^2}}\right)^{\frac12}\\
   &+\|\Delta\vu\|_{L^2} \left(\int_{x_1^2+x_2^2> \gamma} \frac{dx_1dx_2}{16\pi^4\ll_1\ll_2\|\frac{\vx}{\vL}\|^4_{\R^2}}\right)^{\frac12}\\
  &=\|\vu\|_{H^1}  I_1^{\frac12} + \|\Delta\vu\|_{L^2} I_2^{\frac12}.
\end{align*}
By coarea formula:
\[I_1=\int_0^\gamma dr \int_{x_1^2 + x_2^2 = r^2 }\frac{dS}{\ll_1\ll_2 + 4\pi^2\ll_1\ll_2 \|\frac{\vx}{\vL}\|^2_{\R^2}}\]
To compute the latter line intergal along the circle set $x_1=r\sin(t)$ and $x_2=r\cos(t)$:
\begin{align*}
  I_1 &=\int_0^\gamma \int_0^{2\pi} \frac{dr dt}{\ll_1\ll_2 + \frac{4\pi^2}{\ll_1\ll_2}(\ll_2^2 r^2 \sin^2(t)+\ll_1^2 r^2 \cos^2(t))}\\
      &=\int_0^\gamma \frac{dr}{(\ll_1^2+4\pi^2r^2)^{\frac12}(\ll_2^2+4\pi^2r^2)^{\frac12}}\\
      &\le \int_0^\gamma \frac{2\pi rdr}{4\pi^2 r^2+\ll_1\ll_2}=(4\pi)^{-1} \log(1+\frac{4\gamma^2\pi^2}{\ll_1\ll_2})
\end{align*}
Analogously we compute $I_2=\frac{\ll_1^2+\ll_2^2}{32\gamma^2 \pi^3}$. %This completes the proof.
\end{proof}

\begin{proof}
  Take $\oC\in\DtctCls$ and set $\ve=\vu-\vz$. Subtracting \eqref{eq:NSEz} from~\eqref{eq:NSEu} it is easy to get that $\ve$ solves ``the error equation'':  \[
  \dfrac {d}{dt}(\vec e,\vphi) + b(\vec e,\vec u,\vphi) + b(\vec z,\vec e,\vphi) + \nu((\vec e,\vphi)) = (\vf-\vF,\vphi)\eqno(*)
\]
Note that by Poincare inequality~\eqref{eq:Poincare} $\|\nabla\ve\|^2_{\vsLt}=((\ve,\ve))\to0$ implies that $\|\ve\|^2_{\vsLt}=(\ve,\ve)\to 0$ hence, it is sufficient to demonstrate that
$\frac1T\int_t^{t+T} \|\oC\ve(\cdot,s)\|_{\vsLt}ds\to0$ and $\frac1T\int_t^{t+T} \|\vec f(\cdot,s)-\vec F(\cdot,s)\|_{\vsLt}^2 ds \to0$ (conditions $A)$ and $B)$ of Def.~\ref{def:detectability}) imply $V=((\ve,\ve))\to0$ if~\eqref{eq:h-bnd-detect} holds. To this end we plug $\vphi=A\vec e$ into the ``error equation'' $(*)$ and apply simple transformations: (i) recalling from~\eqref{eq:Poincare} and~\eqref{eq:gradA-bnd} that $(\vec e,A\vec e)=((\vec e,\vec e))$, $((\vec e,A\vec e))= (A\vec e,A\vec e)$, and (ii) recalling from~\eqref{eq:b:ort} that $b(\vec e,\vec e, A\vec e)=0$ which implies \(
b(\vec z,\vec e, A\vec e)=b(\vec u-\vec e,\vec e, A\vec e) = b(\vec u,\vec e, A\vec e)
\) so that
\begin{align*}
  b(\vec e,\vec u, A\vec e) &+ b(\vec z,\vec e, A\vec e) = b(\vec e,\vec u, A\vec e) + b(\vec u,\vec e, A\vec e) \\
  &\overset{\cite[F.(A.63)]{NSE-Turbulence-book2001}}{=} -b(\vec e,\vec e, A\vec u)
\end{align*}
we get:
\begin{equation}
      \label{eq:error-Ae}
      \dfrac{d}{dt}((\vec e,\vec e)) + \nu(A\vec e,A\vec e) = (\vf-\vec F,A\vec e) + b(\vec e,\vec e, A\vec u)
\end{equation}
Let us demonstrate that $\nu(A\vec e,A\vec e)$ ``dominates'' $ b(\vec e,\vec e, A\vec u)$ provided that condition $A)$ holds. Indeed
\begin{align*}
     b(\vec e,\vec e, A\vec u) &\overset{\eqref{eq:AgmoN}}{\le} C_1  \log^{\frac12}\bigl(1+\frac{4\pi^2 \gamma^2}{\ll_1\ll_2}\bigr)\|\nabla\ve\|^2_{\vsLt}\|A\vu\|_{\vsLt} \\
                               &+ C_2 \lambda_1^{-1}\gamma^{-1} \|A \vu\|_{\vsLt} \|A\ve\|^2_{\vsLt}
\end{align*}
Now, by~\eqref{eq:InterpIneq}, \eqref{eq:CPoin} and~\eqref{eq:gradA-bnd} we get:
\begin{align}
      \|\nabla\ve\|^2_{\vsLt}
                               %C_{\nabla} (\|\oC\ve\|_{\vsLt}+ h C^{\frac12}_\Omega  \|\nabla\ve\|_{\vsLt})\|A\ve\|_{\vsLt}\\
      &\le  C_{\nabla} (\|\oC\ve\|_{\vsLt}\|A\ve\|_{\vsLt} + h C^{\frac12}_\Omega \lambda_1^{-\frac12} \|A\ve\|^2_{\vsLt})\label{eq:nabla-interp-bnd}
\end{align}
Set $\gamma=\|A \vu\|_{\vsLt} \Gamma$ \textcolor{blue}{for some $\Gamma>0$} and define
\begin{align*}
	\tilde C^1_{h,\Gamma}(t) &= C_1  C_{\nabla} \log^{\frac12}\bigl(1+\frac{4\pi^2 \|A \vu\|_{\vsLt}^2 \Gamma^2}{\ll_1\ll_2}\bigr) h C^{\frac12}_\Omega \lambda_1^{-\frac12}\|A \vu\|_{\vsLt}\\
	&+ C_2 \lambda_1^{-1}\Gamma^{-1}\\
	\tilde C_\Gamma(t) &= C_1  C_{\nabla} \log^{\frac12}\bigl(1+\frac{4\pi^2 \|A \vu\|_{\vsLt}^2 \Gamma^2}{\ll_1\ll_2}\bigr)
\end{align*}
\textcolor{blue}{Using $\tilde C^1_{h,\Gamma}$ and $\tilde C_\Gamma$ and noting that $2\|A\ve\|_{\vsLt}\|A\vu\|_{\vsLt}\le \|A\ve\|^2_{\vsLt}+\|A\vu\|^2_{\vsLt}$ we transform the upper bound for $b$:}
\begin{equation}\label{eq:bUp}
	\begin{split}
		b(\vec e,\vec e, A\vec u)&\le \tilde C^1_{h,\Gamma}(t) \|A\ve\|^2_{\vsLt}\\
        &+ 0.5\tilde C_\Gamma(t) \|\oC\ve\|_{\vsLt}(\|A\ve\|^2_{\vsLt}+\|A\vu\|^2_{\vsLt})
  \end{split}
\end{equation}
By Schwartz inequality:
$$(\vf-\vF,A\ve)\le 1/\nu\|\vf-\vF\|_{\vsLt}^2 + \nu/4(A\ve,A\ve)$$
\textcolor{blue}{We plug the latter inequality and~\eqref{eq:bUp} into~\eqref{eq:error-Ae} (recall that  $V=((e,e))$):
\begin{align}
                  &\dot V + (3\nu/4- \tilde C^1_{h,\Gamma}(t)) (A\vec e,A\vec e)\\
                  &\le \|\vf-\vF\|_{\vsLt}^2/\nu
                  + 0.5\tilde C_\Gamma(t)\|\oC\ve\|_{\vsLt}(\|A\ve\|^2_{\vsLt}+\|A\vu\|^2_{\vsLt})\label{eq:rhsV-detect}
                \end{align}
                If we set $\alpha(t)=(3\nu/4- \tilde C^1_{h,\Gamma}(t))$ and denote by $\beta$ the r.h.s. of~\eqref{eq:rhsV-detect} then $V$ verifies the inequality $\dot V(t) + \alpha(t) V(t) \le \beta(t)$. To show that $V\to0$ we employ Lemma~1.1 from~\cite[p.125]{NSE-Turbulence-book2001}, a generalisation of the classical Gronwall lemma which in our case reads as follows: if $V$ verifies $\dot V(t) + \alpha(t) V(t) \le \beta(t)$ with the just defined $\alpha,\beta$ then $\lim_{t\to\infty}V(t) = 0$ provided there exist $T>0$ such that $\limsup_{t\to\infty}\frac1T\int_t^{t+T} \beta(s) ds =0$ and $\liminf_{t\to\infty}{\frac1T\int_t^{t+T} \alpha(s) ds} >0$. We claim that conditions $A)$ and $B)$ of Def.~\ref{def:detectability} imply the aforementioned condition for $\beta$, and~\eqref{eq:h-bnd-detect} imply the required condition on $\alpha$. To show the former recall from~\cite[p.101, A.60]{NSE-Turbulence-book2001} that} $\sup_{t>t_\Delta}\|A\vu(t)\|_{\vsLt}<C_\Delta$ \textcolor{blue}{for some $C_\Delta >0$ which depends on $\|f\|_{\vsLiHza}$. Similar bound holds for $A\vz$ but depends on $\|F\|_{\vsLiHza}$}. Hence $A\ve = A\vu-A\vz$ is bounded for $t>t_\Delta$ and so is $\tilde C_\Gamma(t)$. \textcolor{blue}{ If conditions $A)$ and $B)$ of Def.~\ref{def:detectability} hold then $\frac1T\int_t^{t+T}\beta(s) ds\to 0$ as $t\to\infty$. Now, to demonstrate condition on $\alpha$ it is sufficient to show that~\eqref{eq:h-bnd-detect} implies
                \begin{equation}
                  \label{eq:C1hnu}
\frac1T\int_t^{t+T} \tilde C^1_{h,\Gamma}(s) ds <(3\nu)/4
\end{equation}}
Indeed, as it follows from~\eqref{eq:Au-ThetatT} and \eqref{eq:Au-L2avrg-bnd} for any $1<\kappa<<2$ there exist $t^\star>0$ and $T>0$ such that \[
  \frac1T\int_t^{T+t}\|A\vu\|^2_{\vsLt}ds  \le \theta_{t,T}\le  \kappa\|\vf\|^2_{\vsLiHza}\nu^{-2}, t>t^\star
  \] \textcolor{blue}{Having this in mind and applying integral Young inequality for
concave function
\begin{equation}
  \label{eq:Young}
  \frac1T\int_t^{t+T}\log(\star)ds\le \log(\frac1T\int_t^{t+T}(\star)ds)
\end{equation}}
we compute:
\begin{align*}
  \frac1T&\int_t^{t+T} \tilde C^1_{h,\Gamma}(s) ds \le C_2 \lambda_1^{-1}\Gamma^{-1} + C_1 C_\nabla h  C^{\frac12}_\Omega \lambda_1^{-\frac12} \theta_{\nu,T}^{\frac12} \times\\
  &\quad \times\bigl(\frac1T\int_t^{t+T}\log\bigl(1+\frac{4\pi^2 \Gamma^2 \|A \vu(t)\|_{\vsLt}^2}{\ll_1\ll_2}\bigr)ds\bigr) ^{\frac12}\\
         &\le C_2 \lambda_1^{-1}\Gamma^{-1} + C_1 C_\nabla h  C^{\frac12}_\Omega \lambda_1^{-\frac12}\kappa^{\frac12}\|\vf\|_{\vsLiHza}/\nu \times\\
  &\qquad \times\log^{\frac12}\bigl(1+\frac{4\pi^2 \kappa \|\vf\|_{\vsLiHza}^2\Gamma^2 }{\nu^2\ll_1\ll_2}\bigr)
\end{align*}
This demonstrates that \eqref{eq:h-bnd-detect} implies~\eqref{eq:C1hnu}.\\
If $\oC\in\DtctClsA$ one needs to invoke~\eqref{eq:CPoin2} in~\eqref{eq:nabla-interp-bnd}, and~\eqref{eq:gradA-bnd} is not required so $\lambda_1^{-\frac12}$ in the r.h.s. of~\eqref{eq:nabla-interp-bnd} disappears as well as in the numerator of~\eqref{eq:h-bnd-detect}.
\end{proof}

\begin{proof}
Note that~\eqref{eq:CPoin} implies that $\oC\in\mathscr{L}(\vsVza)$, and hence the statement of the lemma can be demonstrated by the standard approach to prove existence, uniqueness and regularity for NSE, namely by a combination of a-priori energy bounds and Galerkin projection method. See for example proof of Theorems 5,6 in~\cite{azouani2014continuous} or~\cite[p.192,p.202]{Temam2001}.\\
Analogously~\eqref{eq:CPoin2} implies that $\oC$ is a bounded linear operator on $\dom(A)$, hence by using eigenfunctions of Stokes operator as test functions $\vphi$ in~\eqref{eq:NSE-LO} and the aforementioned  combination of a-priori energy bounds and Galerkin projection method one can prove lemma's statement.
\end{proof}

\begin{proof}
Now, assume that we measure \[
\vec y = \oC(\vu +\vec \psi)
\]
with $\vec\psi=(\psi_1,\psi_2)^\top$ and $\int_\Omega \vec \psi = 0$, provided the noise $\vec\psi=(\eta_1,\eta_2)^\top$ has the following property: the weighted sum of squared averages (somewhat similar to weighted central 2nd moments) of the noise $\eta_{k}$ is bounded \[
\sum_{j=1}^N R_{k,j}\left(\frac1{h^2}\int_{\Omega_j} \eta_k d \vec x\right)^2\le 1, \quad R_{k,j}>0, k=1,2
\]
Let us also assume that  \[
    \oC_1\vu(x,y) = \sum_{j=1}^N\bigl[
\begin{smallmatrix}
  (u_1,\xi_j)\\(u_2,\xi_j)
\end{smallmatrix}\bigr]\frac{\xi_j(x,y)}{h_x^j h_y^j}, \quad \xi_j(x,y)=1, (x,y)\in\Omega_j=(a_j,b_j)\times (c_j,d_j)
\]
with $b_j = a_j+h_x^j$ and $d_j=c_j+h_y^j$. Then~\eqref{eq:CPoin} holds for $h^2=\max_j(\max\{h_x^j,h_y^j\})^2$ and $C_\Omega=(4\pi^2)^{-1}$ by Poincare inequality~\eqref{eq:Poincare}: \[
\|\ve - \oC_1\ve\|_{\vsLt}^2\le h^2 C_\Omega  \|\nabla\ve\|_{\vsLt}^2
\]
For simplicity assume that $h=h_x^j=h_y^j$ so that $h^2 = \int_{\Omega_j} d \vec x$. Take $0<\epsilon<h$ and define a smoothed version of $\oC_1$ given by  \[
      \oC \vec \psi = \sum_{j=1}^N
      \bigl[\begin{smallmatrix}
        \frac1{h}\int_{\Omega_j} \eta_1 d \vec x\\
        \frac1{h}\int_{\Omega_j} \eta_2 d \vec x
      \end{smallmatrix}\bigr]\chi_j
    \]
where the indicator $\xi_j$ is approximated by a piece-wise linear function: \[
     \chi_j (x_1,x_2) = \frac{\chi(x_1,a_j,b_j) \chi(x_2,c_j,d_j)}{h},\quad \chi(x,a,b) =
     \begin{cases}
       \frac{x-a}\epsilon& x\in[a,a+\epsilon]\\
       1& x\in[a+\epsilon,b-\epsilon]\\
       \frac{b-x}\epsilon& x\in[b-\epsilon,b]
     \end{cases}, \quad \epsilon\le (b-a)/2
   \]
   Note that \[
      \int_\Omega \chi^2_j (x_1,x_2) d\vec x = \frac{(h-\frac{4\epsilon}3)^2}{h^2}< 1
    \]
    and \[
      \|\nabla \chi_j\|^2_{\vsLt}=\int_{\Omega_j} \nabla \chi_j\cdot\nabla\chi_j d\vec x = \frac4{\epsilon h} - \frac{16}{3 h^2}
    \]
   In fact
   \begin{align*}
     \|\ve - \oC\ve\|_{\vsLt}&\le  \|\ve - \oC_1\ve\|_{\vsLt}+\|\oC_1\ve - \oC\ve\|_{\vsLt}\\
     &\le \left(h C_\Omega^{\frac12} + \frac{\sqrt{2}(2h\epsilon-\epsilon^2)^{\frac12}}{\sqrt{\lambda_1} h} \right)\|\nabla\ve\|_{\vsLt}\\
     &\le F^{\frac12}(h, \epsilon, C_\Omega) \|\nabla\ve\|_{\vsLt}, \quad F^{\frac12} (h, \epsilon, C_\Omega) =h C_\Omega^{\frac12} + \frac{\sqrt{2}(2h\epsilon-\epsilon^2)^{\frac12}}{\sqrt{\lambda_1} h}
   \end{align*}
   and \[
 \lim_{\epsilon\to0+}F(h, \epsilon, C_\Omega)= 0
   \]
Let $\vu$ solve NSE with $\vf=\vg+\vec d$:
\[
  \dfrac{d}{dt}(\vec u,\vec \phi) + b(\vu,\vu,\vec\phi) + \nu((\vu,\vec \phi)) = (\vg+\vec d,\vec \phi)\,,\vu(0)\in\vsVza
  \]
  and $\vz$ solve observer \[
\dfrac{d}{dt}(\vec z,\vec \phi) + b(\vec z,\vec z,\vec\phi) + \nu((\vec z,\vec \phi)) = (\vec F,\vec \phi)\,, \vz(0)=0
  \]
with \[
      \vF = \vg+L\oC(\vu+\vec \psi) - L \oC \vz = \vg + L \oC \ve + L \oC \vec \psi\,.
    \]

    Then the dynamics of the error $V=((\ve,\ve))$, $\ve=\vu-\vz$ is governed by
    \begin{equation}
      \label{eq:error-Ae1}
      \dfrac{d}{dt}((\vec e,\vec e)) + \nu(A\vec e,A\vec e) = (\vf-\vec F,A\vec e) + b(\vec e,\vec e, A\vec u)
      \end{equation}
      Let us transform~\eqref{eq:error-Ae1}: for any $\Lambda_{1,2}>0$ and $q^2=2\|\vf-\vg\|^2_{\vsLt}=2\|\vec d\|^2_{\vsLt}$ %
   \begin{align}
     (\vf-\vec F,A\vec e) \le& (\vec d + L(\ve-\oC\ve),A\ve) - L(\ve,A\ve)-L(\oC \vec \psi, A\ve) \label{eq:vgLA}\\
                          &+ \Lambda_1(F(h, \epsilon, C_\Omega) \|\nabla\ve\|_{\vsLt}^2 - \|\ve - \oC\ve\|_{\vsLt}^2) \label{eq:vgLA1}\\
                          &+ \Lambda_2(q^2(t) - \|\vec d\|_{\vsLt}^2) \label{eq:vgLA2}
   \end{align}
   where  $\ve = (e_1,e_2)^\top$ and $A\ve=  (-\Delta e_1,-\Delta e_2)^\top$. Note that:
\begin{align*}
      (\oC \vec \psi, A\ve) &= \sum_{j=1}^N \left(\frac1{h}\int_{\Omega_j} \eta_1 d \vec x \int_{\Omega_j}\chi_j(-\Delta e_1)d\vec x  + \frac1{h}\int_{\Omega_j} \eta_2 d \vec x \int_{\Omega_j}\chi_j(-\Delta e_2)d\vec x\right)\\
                                    &\le \sum_{j=1}^N \frac{\sqrt{R_{1,j}}}{h^2}\int_{\Omega_j} \eta_1 d \vec x \frac{h}{\sqrt{R_{1,j}}}\int_{\Omega_j}(\nabla\chi_j\cdot \nabla e_1)d\vec x  + \frac{\sqrt{R_{2,j}}}{h^2}\int_{\Omega_j} \eta_2 d \vec x \frac{h}{\sqrt{R_{2,j}}}\int_{\Omega_j}(\nabla \chi_j\cdot \nabla e_2)d\vec x\\
                                    &\le \sum_{k=1}^2\left(\sum_{j=1}^N \frac{R_{k,j}}{h^4}\left(\int_{\Omega_j} \eta_k d \vec x\right)^2\right)^{\frac12} \left(\sum_{j=1}^N\frac{h^2}{R_{k,j}}\|\nabla\chi_j\|^2_{L^2(\Omega_j)}\|\nabla e_k\|^2_{L^2(\Omega_j)}\right)^{\frac12}\\
                                    &\le \sqrt{2} \left(\sum_{k=1}^2\sum_{j=1}^N\frac{h^2}{R_{k,j}}\|\nabla\chi_j\|^2_{L^2(\Omega_j)}\|\nabla e_k\|^2_{L^2(\Omega_j)}\right)^{\frac12}\\
                                    &\le  \sqrt{2(4h/\epsilon - 16/3)} \left(\sum_{j=1}^N(R^{-1}_{1,j}\|\nabla e_1\|^2_{L^2(\Omega_j)} + R^{-1}_{2,j}\|\nabla e_2\|^2_{L^2(\Omega_j)})\right)^{\frac12}\\
                            &\le \sqrt{2}(4h/\epsilon - 16/3)^{\frac12}\max_k \max_j R^{-\frac12}_{k,j} \|\nabla\ve\|_{\vsLt}\\
  &\le \Sigma^{\frac 12} \|\nabla\ve\|_{\vsLt}, \quad \Sigma_{h,\epsilon,R} = 2(4h/\epsilon - 16/3)\max_k \max_j R^{-1}_{k,j}
\end{align*}
As a result we get: \[
- L(\ve,A\ve)-L(\oC \vec \psi, A\ve) \le -L (\nabla\ve,\nabla \ve) + L \Sigma_{h,\epsilon,R}^{\frac 12} \|\nabla \ve\|_{L^2(\Omega)}
\] and hence for a $\delta<1 $ and $\delta \|\nabla\ve\|_{L^2(\Omega)} > \Sigma_{h,\epsilon,R}^{\frac 12}$ we get: \[
L \Sigma^{\frac 12} \|\nabla \ve\|_{L^2(\Omega)} < L \delta \|\nabla \ve\|^2_{L^2(\Omega)}
\]
and so \[
- L(\ve,A\ve)-L(\oC \vec \psi, A\ve) \le -L (1-\delta) \|\nabla \ve\|^2_{L^2(\Omega)}, \text{ provided } \delta \|\nabla \ve\|_{L^2(\Omega)} > \Sigma_{h,\epsilon,R}^{\frac 12}
  \]
  If $R_{k,j}\equiv \bar R$ then the smallest possible radius of the ``convergence ball'', $\Sigma_{h,\epsilon,R}^{\frac 12}$ is for $\epsilon=h/2$: \[
\Sigma_{h,\epsilon,R}^{\frac 12} = \sqrt{2(8-16/3)/\bar R} = \frac{4}{\sqrt{3\bar R}}
\]
but this (as will be shown below) is possible if for some $\beta<1$:  \[
\beta(1-\delta)^2\Theta(\Gamma_{\max}) C_\Omega >\frac{3}{2\lambda_1}
\]
More generally, the smallest possible radius of the ``convergence ball'' can be found by solving the following optimisation problem:
\begin{align}
  \Sigma_{h,\epsilon,R} &= 2(4h/\epsilon - 16/3)\max_k \max_j R^{-1}_{k,j}\to\min_{h,\epsilon}\\
  &\text{s.t. } h>0, \quad 0<\epsilon\le h/2,\quad  F(h,\epsilon,C_\Omega) \le \beta(1-\delta)^2\Theta(\Gamma_{\max}) C_\Omega
\end{align}
Recall definition of $C_{1,2}$ from~\eqref{eq:C1C2}, and~\eqref{eq:AgmoN}: for any $0<\beta<1$ we have
   \begin{align}
     b(\vec e,\vec e, A&\vec u) \le C_1  \log^{\frac12}\bigl(1+\frac{4\pi^2 \gamma^2}{\ll_1\ll_2}\bigr)\|\nabla\ve\|^2_{\vsLt}\|A\vu\|_{\vsLt}\label{eq:bAgmon} \\
                               &+ (1+\beta - \beta)C_2 \lambda_1^{-1}\gamma^{-1} \|A \vu\|_{\vsLt} \|A\ve\|^2_{\vsLt}\label{eq:bAgmon1}
\end{align}
Set $\gamma=\|A \vu\|_{\vsLt} \Gamma$ with $\Gamma>C_2/(\lambda_1\nu)$, define $\psi_{\Gamma,\nu}=\nu -C_2 /(\lambda_1\Gamma)$, add and substruct $\beta \nu \|A\ve\|^2_{\vsLt}$ to the l.h.s. of~\eqref{eq:error-Ae}, and substitute~\eqref{eq:vgLA}-\eqref{eq:bAgmon1} into r.h.s. of~\eqref{eq:error-Ae}. Collecting the terms with $A\ve$, $\ve-\oC\ve$ and $\vec d$, and transforming the resulting expressions to sums of squares after simple algebra we get:
\begin{align*}
  \dot V &\le \alpha(t)V + \Lambda^*_2q^2(t) -  \|(1-\beta)^\frac12 \psi_{\Gamma,\nu}^{\frac12} A\ve - \sqrt{\Lambda_2^*}\vec d \|^2_{\vsLt}\\
  &- \|\beta^{\frac12} \psi_{\Gamma,\nu}^{\frac12} A\ve - \sqrt{\Lambda_1^*}(\ve-\oC\ve)\|^2_{\vsLt}
\end{align*}
provided $\Lambda^*_1$ solves $\Lambda^*_1 4\beta \psi_{\Gamma,\nu}=L^2$, $\Lambda^*_2$ solves $\Lambda^*_2 4(1-\beta)\psi_{\Gamma,\nu}=1$ and
\begin{align}
%  &\Lambda^*_1= L^2 / (4\beta \psi_{\Gamma,\nu}), \quad \Lambda^*_2=1/((1-\beta)\psi_{\Gamma,\nu})\\
  \alpha &= - L (1-\delta) + \Lambda^*_1 F(h,\epsilon,C_\Omega)+ \Psi(\vu,\Gamma)\label{eq:def:alpha}\\
  \Psi(\vu,\Gamma)&=C_1  \|A \vu\|_{\vsLt}\log^{\frac12}\bigl(1+\frac{4\pi^2 \Gamma^2 \|A \vu\|_{\vsLt}^2}{\ll_1\ll_2}\bigr) \label{eq:def:Psi}
\end{align}
Hence, $\dot V \le \alpha(t)V + \Lambda^*_2q^2(t)$ and by classical Gronwall lemma we have for $t\ge s$:
\begin{equation}
  \label{eq:GBl}
V(t)\le V(s) e^{\int_s^t \alpha(\tau)d\tau} + \Lambda^*_2\int_s^t  q^2(\tau)  e^{\int_\tau^t \alpha(\sigma)d\sigma} d\tau
\end{equation}
Let us shows that 1st and 2nd terms in r.h.s. of~\eqref{eq:GBl} are bounded by the 1st and 2nd terms of~\eqref{eq:ineq-V1} respectively. To bound $e^{\int_s^t \alpha d\tau}$ we show that if $t^\star$ and $T_1$ verify~\eqref{eq:tstarTeps} then for \[
  W(L,\Gamma)= -(1-\delta) L + L^2 F(h,\epsilon,C_\Omega) /(2\beta \hat L_\nabla(\Gamma) C_\Omega) + \hat L_\Delta(\Gamma)
  \] with $\hat L_{\nabla,\Delta}$ defined in~\eqref{eq:hatL}-\eqref{eq:hatL1} it holds:
\begin{align}\label{eq:alphaneg}
\forall t>t^\star: \quad \frac1{T_1}\int_t^{t+T_1}\alpha(s)ds \le W(L,\Gamma)
\end{align}
Indeed, let us take $T_1\ge T$ such that the 2nd term of~\eqref{eq:tstarTeps} is small (e.g. less than $\varepsilon/2$), then note that~\eqref{eq:fgdecay} implies $\lim_{s\to\infty}\Sigma_{T_1}(s)=0$ for any $T_1\ge T$, hence taking a large enough $t^\star$ one can make $\delta(t^\star)$ (1st term of~\eqref{eq:tstarTeps}) and last term of~\eqref{eq:tstarTeps} small enough (e.g. less than $\varepsilon/2$) for~\eqref{eq:tstarTeps} to hold. For these $T_1$ and $t^\star$ we bound $\Psi(\vu,\Gamma)$ defined in~\eqref{eq:def:Psi}: to this end recall integral Young inequality for concave functions~\eqref{eq:Young} which together with~\eqref{eq:Au-L2avrg-bnd} implies for any $T_1>0$
\begin{align}
  \frac1{T_1}\int_t^{t+T_1}\Psi(\vu,\Gamma)ds &\le
                                                %C_1  \theta_{t,T_1}^{\frac12} \bigl(\frac1{T_1}\int_t^{t+T_1}\log\bigl(1+\frac{4\pi^2 \Gamma^2 \|A \vu(s)\|_{\vsLt}^2}{\ll_1\ll_2}\bigr)ds\bigr) ^{\frac12}\\
  C_1  \theta_{t,T_1}^{\frac12}\log^{\frac12}\bigl(1+\frac{4\pi^2 \theta_{t,T_1}\Gamma^2 }{\ll_1\ll_2}\bigr)
  \label{eq:theta:ubnd}
\end{align}
with $\theta_{t,T_1}$ defined in~\eqref{eq:Au-ThetatT}. Now, we bound $\theta_{t,T_1}$: recall definitions of $\kappa$ and $\ball$, and plug $\vf = \vg+\vec d$ into~\eqref{eq:Au-ThetatT}. Noting that $\|\vf\|_{\vsLiHza}\le R+\gnrm$ as $\vec d\in\ball$ we find that 1st term in~\eqref{eq:Au-ThetatT} is bounded by the 2nd term of~\eqref{eq:tstarTeps}, and, by Cauchy-Schwartz inequality, the 2nd term in~\eqref{eq:Au-ThetatT} is bounded by $\frac{\gnrm^2}{\nu^2}+\delta(t^\star)$ hence by~\eqref{eq:tstarTeps}:
    \begin{equation}
    \label{eq:Thetabnd}
    \begin{split}
      \theta_{t,T_1} &\le \bigl(\frac{2(\gnrm+R)^2}{\gnrm^2 T_1\nu\lambda_1} + \frac{2\nu\mathbb{e}^{-\lambda_1 \nu t}\|\nabla\vec u_0\|^2_{\vsLt}}{T_1 \gnrm^2} +\delta\bigr)\times\\
      &\times\frac{\gnrm^2}{\nu^2}+ \frac{\gnrm^2}{\nu^2}\le  \kappa \frac{\gnrm^2}{\nu^{2}},\,t>t^\star, T_1\ge T
    \end{split}
  \end{equation}
  Substituting~\eqref{eq:def:alpha}, \eqref{eq:theta:ubnd} and~\eqref{eq:Thetabnd} into l.h.s. of~\eqref{eq:alphaneg}, noting that $\Lambda^*_1=L^2/(4\beta\psi_{\Gamma,\nu})$ and recalling definition of $\hat L_\nabla$ we obtain~\eqref{eq:alphaneg}.

\textcolor{blue}{Let us show that $W(L,\Gamma)<0$ for some $h$ and $L$. Indeed, $W$ is a quadratic polynomial (in $L$) with two distinct real roots \[
    L_\pm=\frac{1-\delta \pm\sqrt{(1-\delta)^2-4  a \hat L_\Delta}}{2a}, \quad a =  F(h,\epsilon,C_\Omega)/(2\beta \hat L_\nabla(\Gamma)C_\Omega)
  \]
  provided the discriminant of $W$ is positive: $(1-\delta)^2-4a \hat L_\Delta> 0$. The latter implies $0<L_-<L_+$ and since $W(0,\Gamma) =\hat L_\Delta>0$ it follows that $W(L,\Gamma)<0$ for any $L\in(L_-,L_+)$. Hence, $W(L,\Gamma)<0$ for \[
    L=\beta(1-\delta)\hat L_\nabla C_\Omega/F(h,\epsilon,C_\Omega)= (L_++L_-)/2 \in (L_-,L_+)
  \]
  provided $4a \hat L_\Delta<(1-\delta)^2$ which is the case for \[
    F(h,\epsilon,C_\Omega)< (1-\delta)^2(2\beta \hat L_\nabla(\Gamma) C_\Omega)/(4 \hat L_\Delta(\Gamma))=(1-\delta)^2\beta \Theta(\Gamma) C_\Omega
  \]
Specifically, $W(L, \Gamma_{\mathrm{max}} )=Q(L)<0$ for $Q(L)$ defined in~\eqref{eq:ineq-V1}, and $\omega$, $L$ chosen as in $C1)$, and in fact choosing $\Gamma = \Gamma_{\mathrm{max}}$ allows to maximize the upper-bound for $h^2$. Hence, $\forall t>t^\star$ and $\omega=1/2$, $ L =(1-\delta)\beta\hat L_\nabla(\Gamma_{\mathrm{max}}) /h^2$:
\begin{equation}
  \label{eq:alpha-QL}
\frac1{T_1}\int_t^{t+T_1}\alpha(s)ds \le Q(L)<0
\end{equation}
Now we are ready to bound $e^{\int_s^t \alpha d\tau}$. To this end we follow the derivation from~\cite[p.156, f.(A.4)]{NSE-Turbulence-book2001}, namely the argument given after formula (A.3) there: take an integer $k=\lfloor\frac{t-s}{T_1}\rfloor$, that is the smallest integer $k\ge0$ such that $s+kT_1\le t\le s+(k+1)T_1$, and note that
\begin{equation}
  \label{eq:exp-alpha-bnd}
  \begin{split}
    &e^{\int_s^t \alpha(\tau)d\tau}=  e^{\int_s^{s+kT_1} \alpha(\tau)d\tau}e^{\int_{s+kT_1}^t \alpha(\tau)d\tau }\\
    &\overset{\eqref{eq:alpha-QL},\eqref{eq:def:alpha}}{\le} e^{Q(L)T_1 k } e^{-L\omega(t-s-kT_1)+\int_{s+kT_1}^{s+(k+1)T_1} \Psi(\vu,\Gamma_{\mathrm{max}})d\tau }\\
    &\le e^{Q(L) T_1(k+1)}e^{-T_1Q(L)}  e^{-L\omega(t-s-kT_1) + T_1 \hat L_\Delta(\Gamma_{\mathrm{max}})}\\
    &\le e^{(Q(L)-\omega L)(t-s) + \omega L T_1\lfloor\frac{t-s}{T_1}\rfloor}e^{\omega LT_1}
  \end{split}
\end{equation}
where to go from 2nd to 3rd line of~\eqref{eq:exp-alpha-bnd} we employed \eqref{eq:theta:ubnd},\eqref{eq:Thetabnd},\eqref{eq:hatL1}, and from 3rd to 4th -- $e^{T_1 (k+1) Q(L)}\le e^{Q(L)(t-s)}$ (as $Q(L)<0$ and $t-s\le(k+1)T_1$).}

\textcolor{blue}{Now, let us bound the 2nd term of~\eqref{eq:GBl}. Again, we follow the derivation of~\cite[p.156, f.(A.5)]{NSE-Turbulence-book2001}, namely the argument given after formula (A.4) there, which is based on exponential sum formulas:
\begin{equation}
  \label{eq:qbnd}
\int_s^t  q^2(\tau)e^{\int_\tau^t \alpha(\sigma)d\sigma} d\tau \le 2 T_1 e^{T_1 (\omega L - Q(L))}\Sigma_{T_1}(s)
\end{equation}
Finally, recalling~\eqref{eq:hatL} and definition of $\Lambda_2^\star$ we deduce~\eqref{eq:ineq-V1} from \eqref{eq:GBl}, \eqref{eq:exp-alpha-bnd} and \eqref{eq:qbnd}.}

\textcolor{blue}{Now, let us demonstrate that $C2)$ implies~\eqref{eq:ineq-V1}.} If $\oC\in\DtctClsA$ then~\eqref{eq:vgLA1} changes to $\Lambda_1(h^2 C_\Omega \|A\ve\|_{\vsLt}^2 - \|\ve - \oC\ve\|_{\vsLt}^2)$ as it follows from~\eqref{eq:CPoin2}. Now, as above (\textcolor{blue}{see discussion right after~\eqref{eq:bAgmon1}}), we substitute~\eqref{eq:vgLA}, modified~\eqref{eq:vgLA1} and~\eqref{eq:vgLA2}-\eqref{eq:bAgmon1} into r.h.s. of~\eqref{eq:error-Ae}, and collect terms with $A\ve$, $\ve-\oC\ve$ and $\vec d$:
\begin{align*}
  \dot V &\le \alpha'(t)V + \Lambda^\star_2q^2(t) -  \|(1-\beta)^\frac12 \psi_{\Gamma,\nu}^{\frac12} A\ve - \sqrt{\Lambda_2^*}\vec d \|^2_{\vsLt}\\
         &- \|(\beta\psi_{\Gamma,\nu}-\Lambda'_1 h^2 C_\Omega)^{\frac12}A\ve - \sqrt{\Lambda_1'}(\ve-\oC\ve)\|^2_{\vsLt}
\end{align*}
provided \textcolor{blue}{$\Lambda^*_2$ solves $\Lambda^*_2 4(1-\beta)\psi_{\Gamma,\nu}=1$ (as above)}, and
\begin{equation}
  \label{eq:alpha-prime}
\alpha' =  - L + \Psi(\vu,\Gamma) %C_1  \|A \vu\|_{\vsLt}  \log^{\frac12}\bigl(1+\frac{4\pi^2 \Gamma^2 \|A \vu\|_{\vsLt}^2}{\ll_1\ll_2}\bigr)
\end{equation}
\textcolor{blue}{and $\Lambda_1'$ solves a quadratic equation $4\Lambda_1(\beta\psi_{\Gamma,\nu}-\Lambda_1 h^2 C_\Omega) = L^2$, solution of which is given by:
\begin{align}
  \Lambda_1' &= \frac{\psi_{\Gamma,\nu}+\sqrt{\beta^2\psi_{\Gamma,\nu}^2-L^2 C_\Omega h^2}}{2h^2 C_\Omega}\\
  &\text{provided: }\psi_{\Gamma,\nu}>0, \quad L h\sqrt{C_\Omega} < \beta\psi_{\Gamma,\nu}\label{eq:Lambdaprime}
\end{align}}
%and this formula makes sence if $\psi_{\Gamma,\nu}>0$ and $L h\sqrt{C_\Omega} < \beta\psi_{\Gamma,\nu}$.
Hence $\dot V \le \alpha'(t)V + \Lambda^\star_2q^2(t)$, provided~\eqref{eq:Lambdaprime} holds. \textcolor{blue}{Analogously to what has been done above, to demonstrate~\eqref{eq:ineq-V1} one can repeat all the steps given after \eqref{eq:def:Psi}: employ GB-lemma to derive analog of~\eqref{eq:GBl}, and then bound its terms. Since the last term is the same, the only bound that remains to be established is the analog of~\eqref{eq:alpha-QL}, namely that $\frac1{T_1}\int_t^{t+T_1}\alpha'(s)ds < Q(L)=-L\omega + \hat L_\Delta(\Gamma_{\mathrm{max}})<0$ for $L$ and $\omega$ defined in $C2)$. But the first part of the latter inequality immediately follows from~\eqref{eq:alpha-prime} and \eqref{eq:theta:ubnd}, \eqref{eq:Thetabnd}, \eqref{eq:hatL1}, and the inequality $Q(L)<0$ holds if $L=\theta\hat L_\Delta(\Gamma_{\mathrm{max}})$ for $\theta>1$ (as suggested in $C2)$). To satisfy~\eqref{eq:Lambdaprime} we set $\Gamma=\Gamma_{\mathrm{max}}$ and substitute $L=\theta\hat L_\Delta(\Gamma_{\mathrm{max}})$ into~\eqref{eq:Lambdaprime} and get a condition on $h: h < \frac{\beta\psi_{\Gamma,\nu}}{\theta \hat L_\Delta\sqrt{C_\Omega}}=\beta \sqrt{C_\Omega} \theta^{-1} \Theta(\Gamma)$ as suggested in $C2)$. Note that $\Gamma_{\mathrm{max}}>C_2/(\lambda_1\nu)$ hence $\psi_{\Gamma_{\mathrm{max}},\nu}>0$ as required by~\eqref{eq:Lambdaprime}. Hence, ~\eqref{eq:ineq-V1} holds for $V$ if $L$, $\omega$ and $h$ are defined as in $C2)$. This completes the proof.}
% \textcolor{blue}{To prove the last statement, we note that $V$ is indeed asymptotically proportional to $\frac1{T} \int_t^{t+T} q^2(s)ds$ with constant depending on $T$ (see proof of Lemma 1.1 in~\cite[p.157]{NSE-Turbulence-book2001}), provided $\vec d\ne 0$. Assume that $\vec d(s)=0$ in $L^2(\Omega)$ for $s>s^\star$ and let $C1)$ hold. Then obviously $q_2=0$ and so $\forall t>\max\{t^\star,s^\star\}$ \[
%     V(t+\bar T)\le e^{\int_t^{t+\bar T} \alpha(s) ds}V(t)\le e^{Q(\beta \hat L_\nabla / h^2) \bar T} V(t)
%   \]
%   provided $t^\star,\bar T$ verify~\eqref{eq:tstarTeps}. $C1)$ guarantees that $\xi=Q(\beta \hat L_\nabla / h^2)<0$. $C2)$ implies similar bound on $V(t+T)$. If $\|\nabla\vec u_0\|^2_{\vsLt}\le C_0$ $t^\star$ and $\bar T$ can be computed as suggested in the theorem. This completes the proof.}
\end{proof}

%%% Local Variables:
%%% mode: latex
%%% TeX-master: "main-noisy-obs"
%%% End:
